# Supplementary material for: Event-Based Visual Odometry on Non-Holonomic Ground Vehicles
Source: arXiv:2401.09331 source file (2024-01-17)
Supplement: Supplementary file 1 [file X_suppl.tex]

\clearpage
\setcounter{page}{1}
\maketitlesupplementary

\section{$a_{ij}$ for \textit{s5c4} and \textit{s7c6}}
For \textit{s5c4}, we have
\begin{scriptsize}
\begin{equation*}
\begin{split}
    a_{i1} \approx \widetilde{a}_{i1} = 
    & - x_i(\frac{(\omega\Delta t_i)^5}{120} -
    \frac{(\omega\Delta t_i)^3}{6} + \omega\Delta t_i)\\
    & + \frac{(\omega\Delta t_i)^4}{24} -  \frac{(\omega\Delta t_i)^2}{2} + 1,\\
    a_{i2} \approx \widetilde{a}_{i2} = 
    &  - x_i(\frac{(\omega\Delta t_i)^4}{24} - \frac{(\omega\Delta t_i)^2}{2} + 1)\\
    & - \frac{(\omega\Delta t_i)^5}{120} + \frac{(\omega\Delta t_i)^3}{6} - \omega\Delta t_i ,\\
    a_{i3} \approx \widetilde{a}_{i3} =
    &  \frac{\Delta t_i(x_i\Delta t_i^4\omega^4 - 5\Delta t_i^3\omega^3 - 20x_i\Delta t_i^2\omega^2 + 60\Delta t_i\omega + 120x_i)}{\tau(\tau^4\omega^4 - 20\tau^2\omega^2 + 120)}.
\end{split}
\end{equation*}
\end{scriptsize}
For \textit{s7c6} we obtain
\begin{scriptsize}
\begin{equation*}
\begin{split}
    a_{i1} \approx \widetilde{a}_{i1} = 
    & x_i(\frac{(\omega\Delta t_i)^7}{5040} - \frac{(\omega\Delta t_i)^5}{120} + \frac{(\omega\Delta t_i)^3}{6} - \omega\Delta t_i)  \\ 
    &  - \frac{(\omega\Delta t_i)^6}{720} + \frac{(\omega\Delta t_i)^4}{24} - \frac{(\omega\Delta t_i)^2}{2} + 1,\\
    a_{i2} \approx \widetilde{a}_{i2} = 
    & x_i(\frac{(\omega\Delta t_i)^6}{720} - \frac{(\omega\Delta t_i)^4}{24} + \frac{(\omega\Delta t_i)^2}{2} - 1) \\
    & + \frac{(\omega\Delta t_i)^7}{5040} - \frac{(\omega\Delta t_i)^5}{120} + \frac{(\omega\Delta t_i)^3}{6} - \omega\Delta t_i,\\
    a_{i3} \approx \widetilde{a}_{i3} = 
    & \frac{-(\Delta t_i(- x_i\Delta t_i^6\omega^6 + 7\Delta t_i^5\omega^5 + 42x_i\Delta t_i^4\omega^4 - 210\Delta t_i^3\omega^3}{\tau(\tau^6\omega^6 - 42\tau^4\omega^4 + 840\tau^2\omega^2 - 5040)}\\
    & \frac{-(\Delta t_i(- 840x_i\Delta t_i^2\omega^2 + 2520\Delta t_i\omega + 5040x_i))}{\tau(\tau^6\omega^6 - 42\tau^4\omega^4 + 840\tau^2\omega^2 - 5040)}.
\end{split}
\end{equation*}
\end{scriptsize}
